# Supplementary material for: Leveraging Uncertainty Estimates To Improve Classifier Performance
Source: arXiv:2311.11723 source file (2023-11-20)
Supplement: Supplementary file 1 [file appendix_analysis.tex]

\section{Details on Estimation Bias Analysis}
\label{appendix:analysis}

% O: Theorem 2.1 with proof
\begin{theorem} {\bf [Restatement of Theorem \ref{thm:bias}]}
Under Assumption 2.1 and a differential sampling of $\frac{1}{\tau}$, the estimation bias in the model score for the positive class  from Posterior Networks at $\x$  is given by
$$ \frac{e(s) +f(s)\gamma(\x)}{g(s)+h(s)\gamma(\x)}, $$ 
where $s=s(\x)$ denotes the model score and 
\begin{itemize}
\item  $\omega =\frac{\beta_1^{prior}}{\beta_1^{prior} + \beta_0^{prior}}$ denotes the positive class prior ratio,  
\item $\gamma(\x)  =  \frac{\beta_1^{prior} + \beta_0^{prior}} {\beta_1(x) + \beta_0(x)}$  denotes the relative strength of priors to evidence
\item $e(s) = s(1-s)(\tau-1)$; $~~f(s) = (1 + s(\tau -1))(w-s)$
 \item $g(s) = \tau - s(\tau-1)$; $~~h(s) = (\tau -1)(w-s) $.
\end{itemize}
\end{theorem}

\proof 
From Bayes rule, using Assumption 2.1 and adjusting for the differential sampling,  the positivity rate at $\x$ in the test dataset is  given by
\begin{eqnarray*}
s^{emp-test}(\x) &=& \pr(y=1|\x) =  \frac { \pr_{test}(y=1) \pr(\x | y=1)} {  \sum_{c=0,1} \pr_{test}(y=c) \pr(\x |y=c) } \\
&=& \frac{ \beta_1(\x) } { \beta_1(\x) + \tau \beta_0(\x)}. 
\end{eqnarray*}

Let  $\omega =\frac{\beta_1^{prior}}{\beta_1^{prior} + \beta_0^{prior}}$ denote the positive class prior ratio and  
$\gamma(\x)  =  \frac{\beta_1^{prior} + \beta_0^{prior}} {\beta_1(x) + \beta_0(x)}$  denote the relative strength of priors to evidence. To simplify the computation of  the estimation bias $(s(\x) - s^{emp-test} (\x))$,  we define an additional auxiliary variable 
$\kappa(\x) = \frac{\beta_1(\x) }{\beta_1(\x) + \beta_0(\x)}$, which corresponds to the train positivity rate.  We then obtain $\beta_0(\x) =  \beta_1(x) \big(\frac{ 1- \kappa(\x)} {\kappa(\x)}\big)$.

The model score $s(\x)$ can now be expressed in terms of $\omega, \kappa(\x)$ and $\gamma(\x)$ as follows:
\begin{equation}
s(\x) =  \frac{ \beta_1^{prior} +  \beta_1(\x) } { \sum_{c \in \cC} [\beta_c^{prior} +  \beta_c(\x)] } 
 = \frac{ \omega\gamma(x) + \kappa(\x)} {1+ \gamma(x)}.
 \label{ref:eqn4}
\end{equation}
Hence, $\kappa(\x) = s(x) - (\omega -s(\x)\gamma(\x)$. The estimation bias with respect to the test positivity rate is given by
\begin{eqnarray*}
s(\x) - s^{emp-test} (\x) &=& s(\x) - \frac{ \beta_1(\x) } { \beta_1(\x) + \tau \beta_0(\x)}  \\
&=& s(\x) - \frac{ \beta_1(\x) } { \beta_1(\x) + \beta_1(\x) \tau \big(\frac{1-\kappa(\x)}{\kappa(\x)}\big)} \\
&=& s(\x) - \frac{ 1} {1 + \tau \frac{1-\kappa(\x)}{\kappa(\x) }} \\
%&=& \frac{ s(x) ( \kappa(\x)  +  \tau(1- \kappa(x) ) )   - \kappa(\x) } {  \kappa(\x)  +  \tau(1- \kappa(x) ) } \\
&=& \frac{ s(x) ( \kappa(\x)  +  \tau(1- \kappa(x) ) )   - \kappa(\x) } {  \kappa(\x)  +  \tau(1- \kappa(x) ) }. \\
\end{eqnarray*}

Denoting $s(\x), \kappa(x)$ and $(\omega - s(\x)) \gamma(\x)$  by $s, \kappa, v$ for brevity, we have $\kappa =s - v$. The estimation bias can be simplified as 
\begin{eqnarray*}
s(\x) - s^{emp-test} (\x) &=& \frac{ s ( \kappa  +  \tau(1- \kappa ) )   + \kappa } {  \kappa  +  \tau(1- \kappa ) } \\
&=& \frac{ s( s-v + \tau (1-s+v) )  - s+v }  {s-v + \tau (1-s+v)} \\
&=& \frac{  s(s +\tau(1-s) -1)      +v (s\tau - s  +1) } {s + \tau(1-s)  + v (\tau-1) }\\
%&=& \frac{ s(1-s)(\tau-1) + v (1+ s(\tau-1))}{\tau  -  s(\tau-1)  + v (\tau-1) }\\
&= &  \frac{e(s) +f(s)\gamma(\x)}{g(s)+h(s)\gamma(\x)}, 
\end{eqnarray*}
where we have
\begin{itemize}
\item $e(s) = s(1-s)(\tau-1); ~~~ f(s) = (1 + s(\tau -1))(w-s)$
 \item $g(s) = \tau - s(\tau-1); ~~~ h(s) = (\tau -1)(w-s) $.
\end{itemize}
\qed

%O: result - fixed score behavior
\begin{corollary}
For a fixed choice of score $s(\x)$, the estimation bias has an increasing or decreasing trend with respect to $\gamma(\x)$  (and thereby uncertainty) depending on whether $(s(\x)  <\omega)$ or $(s(\x) > \omega)$.
\label{thm:fixedscore}
\end{corollary}
\proof 
Denoting $s=s(\x)$ and $\gamma = \gamma(\x)$ for brevity, the first order partial derivative of the estimation bias with respect to uncertainty $\gamma$ is given by
\begin{eqnarray*}
\frac{d}{d\gamma}\bigg( 
\frac{e(s)+f(s)\gamma}{g(s)+h(s)\gamma} \bigg)  
&= & \frac{-(e(s) +f(s)\gamma)h(s) + (g(s) + h(s)\gamma)f(s)} 
{(g(s)+h(s)\gamma)^2} \\
&= & \frac{-e(s)h(s) + f(s)g(s)}{(g(s)+h(s)\gamma)^2}  \\
&=&  \frac{\omega-s} {(g(s)+h(s)\gamma)^2} \big (1 + s(\tau -1) )(\tau - s(\tau-1)) - s(1-s)(\tau-1)^2  \big) \\
&=&  \frac{\tau (\omega -s)} {(g(s)+h(s)\gamma)^2}. \\
\end{eqnarray*}

Since $\frac{\tau}{(g(s)+h(s)\gamma)^2} >0$ for all choices of $\tau$ and model score values, the sign of the first order derivative depends on whether $s(\x)  <\omega$ or $s(\x) > \omega$. Hence, for the lower score range, the estimation bias increases monotonically with the uncertainty level while it decreases with uncertainty in a higher score range. 
Note that the trend described is for the value of the estimation bias disregarding the sign and magnitude. 
Since estimation bias is the difference between the model score and the  true test positivity rate, the trend with respect to the test positivity rate is opposite of the one with respect to estimation bias. 
\qed

%O: result - fixed uncertainty behavior
\begin{corollary}
For a fixed choice of uncertainty $\gamma(\x)$, (a) the true test positivity rate in Theorem \ref{thm:bias} is monotonically increasing in the score, and 
(b)  the valid score range is limited to 
$ [ \frac{ \omega\gamma(x)} {1+ \gamma(x)}, ~ \frac{ 1+ \omega\gamma(x)} {1+ \gamma(x)} ]$.
\label{thm:fixedunc}
\end{corollary}

\proof
(a) Denoting $s=s(\x)$ and $\gamma = \gamma(\x)$ for brevity, the first order partial derivative of the test positivity rate with respect to score $\gamma$ is given by
\begin{eqnarray*}
\frac{ds^{emp-test}(\x)}{ds} )  
&=& \frac{d}{ds} \bigg( s - \frac{e(s)+f(s)\gamma}{g(s)+h(s)\gamma} \bigg)   \\
&= &  1 - \frac{1} {(g(s)+h(s)\gamma)^2}  [ (g(s) + h(s)\gamma) (e’(s) + f’(s)\gamma) -  (e(s) + f(s)\gamma) (g’(s) + h’(s)\gamma) ]  \\
\end{eqnarray*}
where $e’(s), f’(s), g’(s), h’(s)$ denote the derivatives of $e(s), f(s), g(s), h(s)$ respectively with respect to score and are given by
\begin{itemize}
\item $e’(s) = (\tau-1)(1-2s); ~~ f’(s) =  (\tau -1)(w -2s);$ 
\item $~~g’(s) = - (\tau-1); ~~h’(s) = - (\tau -1).$
\end{itemize}

Substituting these and using $\chi=(\tau-1) >0 $ for brevity  we obtain
\begin{eqnarray*}
\frac{ds^{emp-test}(\x)}{ds}  
&=&   \frac{1} {(g(s)+h(s)\gamma)^2}  \bigg[ (g(s) + h(s)\gamma) ( g(s) + h(s)\gamma  - \chi (1+ \omega\gamma -2s(1+\gamma)  )  -  (e(s) + f(s)\gamma) \chi(1+ \gamma) \bigg]  \\
%&=&   \frac{1} {(g(s)+h(s)\gamma)^2} \bigg[ (g(s) + h(s)\gamma) (1 + \chi s(1+ \gamma) )  -  (e(s) + f(s)\gamma) \chi(1+ \gamma) \bigg]  \\
&=&   \frac{1} {(g(s)+h(s)\gamma)^2}  \bigg[ (g(s) + h(s)\gamma)   -  \chi (1+ \gamma)  (e(s) + f(s)\gamma  - sg(s) -sh(s)\gamma)  \bigg]  \\
%&=&   \frac{1} {(g(s)+h(s)\gamma)^2}  \bigg[ (g(s) + h(s)\gamma)   -  \chi (1+ \gamma)  (e(s) + f(s)\gamma  - sg(s) -sh(s)\gamma)  \bigg]  \\
&=&   \frac{1} {(g(s)+h(s)\gamma)^2}  \bigg[ (g(s) + h(s)\gamma)   -  \chi (1+ \gamma) (\gamma-s) \bigg]  \\
%&=&   \frac{1} {(g(s)+h(s)\gamma)^2}  \bigg[ 1+ \chi - s\chi(1+\gamma) + \chi\omega\gamma   -  \chi (1+ \gamma) (\gamma-s) \bigg]  \\
%&=&   \frac{1} {(g(s)+h(s)\gamma)^2}  \bigg[ 1 + \chi +  \chi\omega\gamma   -  \chi\gamma(1+\gamma) \bigg]  \\
&=&   \frac{1} {(g(s)+h(s)\gamma)^2}  \bigg[ 1 + \chi (1-\gamma)^2  + \chi\gamma(1+\omega) \bigg]  \\
& > &  0  ~~ \{ ~~~\text{since the Nr is at least 1 and the Nr is positive as well} \}. \\
\end{eqnarray*}
Hence, for a fixed uncertainty level,  empirical positivity rate is always monotonically increasing with score even in case of undersampling despite the estimation bias. 

(b)  Given $\omega$ and $\gamma =\gamma(\x)$, the model output score is least for any $\x$ when the evidence does not have any support for the positive class, i.e., $\beta_1(\x) =0$  and  $\kappa(\x) =0$ . The score is maximum at any point $\x$ where the evidence has maximal support for the positive class, i.e., $\beta_0(\x)=0$ and  $\kappa(\x) =1$. From Eqn. (\ref{ref:eqn4}), we observe that   $s(\x) = \frac{ \omega\gamma(x) + \kappa(\x)} {1+ \gamma(x)}$. Hence, the valid range for score for a given $\omega, \gamma(x)$  is given by   $ [ \frac{ \omega\gamma(x)} {1+ \gamma(x)}, ~ \frac{ 1+ \omega\gamma(x)} {1+ \gamma(x)} ]$. When $\gamma(\x)$ is small, the permissible score range is broader  and narrows as $\gamma(\x)$ increases.
\qed
